# Supplementary material for: Towards Automated Solution Recipe Generation for Industrial Asset Management with LLM
Source: arXiv:2407.18992 source file (2024-07-26)
Supplement: Supplementary file 1 [file appendix_claims.tex]

\section{Claims Identified for Wind Turbine Health}
\vspace{10pt}

\begin{table}[!ht]
    \centering
    \begin{tabular}{|l|l|l|}
    \hline
        PassageID & Part & Claim \\ \hline
        1 & asset description & A wind turbine converts the kinetic energy of wind into electrical energy by first converting it into mechanical energy. \\ \hline
        1 & asset description & "Wind turbines are used in various applications, including power generation, water pumping, and sailing." \\ \hline
        1 & asset description & "The main components of a wind turbine include the rotor blades, the hub, the main shaft, the gearbox, the generator, the yaw system, and the control system." \\ \hline
        2 & component condition & "The condition of wind turbine blades, including any damage from erosion, lightning strikes, or collisions, can impact the efficiency and risk of failure in a wind turbine." \\ \hline
        2 & component condition & "The generator, gearbox, main bearing, and yaw system of a wind turbine can all experience wear, damage, or degradation that can lead to failure, and therefore require regular monitoring and maintenance." \\ \hline
        2 & component condition & "Excessive noise or leakage from a wind turbine can indicate underlying mechanical issues, such as loose bearings or imbalanced rotors, and should be investigated to prevent potential failures." \\ \hline
        3 & Sensor Measurement & "Visual inspections and LiDAR sensors can be used to monitor the condition of wind turbine blades, and can help identify any signs of damage or wear, as well as changes in the blade's aerodynamic performance." \\ \hline
        3 & Sensor Measurement & "Temperature sensors, vibration sensors, and current sensors can be used to monitor the condition of a wind turbine generator, and can help identify issues with the thermal performance, mechanical components, and electrical components of the equipment." \\ \hline
        3 & Sensor Measurement & "Oil analysis sensors, vibration sensors, temperature sensors, and displacement sensors can be used to monitor the condition of a wind turbine gearbox and main bearing, and can help identify issues with the mechanical components and thermal performance of the equipment." \\ \hline
    \end{tabular}
\end{table}
