# Supplementary material for: Towards Automated Solution Recipe Generation for Industrial Asset Management with LLM
Source: arXiv:2407.18992 source file (2024-07-26)
Supplement: Supplementary file 2 [file appendix_artifacts.tex]

\begin{comment}

\section{Generated Artifacts}
\vspace{10pt}

In this section, we provided a limited number of artifacts as a demonstration of the capability of our system. It is also part of the validation of the usefulness of this approach in the rapid development of a solution.

In this section, we will display the artifact generated for a given asset class, ten asset classes.

\begin{markdown}
# Wind Turbine Health Guideline

*Remember* to grab as much as we can during upcoming [sales](http://acme-marg.com)!

## Food

- baked beans
- spaghetti

## Stationery 

- writing pad
- pencils
\end{markdown}
    
\end{comment}
